# Supplementary material for: Paint and Distill: Boosting 3D Object Detection with Semantic Passing Network
Source: arXiv:2207.05497 source file (2022-07-12)
Supplement: Supplementary file 2 [file appendix_table2.tex]

\begin{table}[t]
 \caption{Loss weight combinations in the SPNet-P for the car class at IOU=0.7 (R11) on KITTI validation set.}
 \centering
 \begin{tabular}{c|ccc|ccc}
  \toprule
   \multirow{2}{*}{Group} & $\mathcal{L}_c$      & $\mathcal{L}_f$      & $\mathcal{L}_p$      & \multicolumn{3}{c}{3D Detection (\%)}     \\
   & loss     & loss     & loss           & Mod.                & Easy                 & Hard    \\
  \hline
  \uppercase\expandafter{\romannumeral1} & 0       & 0      & 0      & 77.31       & 87.29        & 75.55         \\
%   \uppercase\expandafter{\romannumeral2} & 0       & 1      & 10     & 78.22       & 88.42        & 76.74         \\
  \uppercase\expandafter{\romannumeral2} & 0       & 10     & 10     & 78.28       & 88.65        & 76.86         \\
  \uppercase\expandafter{\romannumeral3} & 1       & 1      & 10     & 78.31       & 87.88        & 77.08         \\
  \uppercase\expandafter{\romannumeral4} & 0.01    & 1      & 10     & 78.20       & 88.12        & 76.70         \\
  \uppercase\expandafter{\romannumeral5} & 0.1     & 10     & 10     & \textbf{78.67} & \textbf{88.71} & \textbf{77.29}\\
  \bottomrule
 \end{tabular}
 \label{appendix_loss_exp_p}
\end{table}
