# Supplementary material for: Paint and Distill: Boosting 3D Object Detection with Semantic Passing Network
Source: arXiv:2207.05497 source file (2022-07-12)
Supplement: Supplementary file 3 [file appendix_table3.tex]

\begin{table}[t]
 \caption{Loss weight combinations in the SPNet-V for the car class at IOU=0.7 (R11) on KITTI validation set.}
 \centering
 \begin{tabular}{c|ccc|ccc}
  \toprule
   \multirow{2}{*}{Group} & $\mathcal{L}_c$      & $\mathcal{L}_f$      & $\mathcal{L}_p$      & \multicolumn{3}{c}{3D Detection (\%)}     \\
   & loss     & loss     & loss           & Mod.                & Easy                 & Hard    \\
  \hline
  \uppercase\expandafter{\romannumeral1} & 0       & 0      & 0      & 76.98       & 86.76        & 74.54         \\
%   \uppercase\expandafter{\romannumeral2} & 0.1     & 10     & 10     & 77.97       & 87.81        & 76.82         \\
  \uppercase\expandafter{\romannumeral2} & 0.1     & 1      & 10     & 78.20       & \textbf{88.34}        & 77.01         \\
  \uppercase\expandafter{\romannumeral3} & 1       & 10     & 20     & 78.29       & 88.18        & 77.21         \\
  \uppercase\expandafter{\romannumeral4} & 10      & 10     & 10     & 78.20       & 87.81        & 77.07         \\
  \uppercase\expandafter{\romannumeral5} & 1       & 10     & 10     & \textbf{78.32} & 87.88 & \textbf{77.24}\\
  \bottomrule
 \end{tabular}
 \label{appendix_loss_exp_v}
\end{table}
